# Supplementary material for: HHGT: Hierarchical Heterogeneous Graph Transformer for Heterogeneous Graph Representation Learning
Source: arXiv:2407.13158 source file (2024-07-18)
Supplement: Supplementary file 1 [file appendix.tex]

\section{Dataset Description}
\label{sec:dataset}
The details of three HIN benchmark datasets used in this paper are described as follows. 

\begin{itemize}[leftmargin=*]
\item \textbf{IMDB} is extracted from the online film rating website, which contains 3,228 movies (M), 42,553 actors (A), 2,103 users (U) and 2,016 directors (D). All types of nodes are associated with 128-dimension features. There are three relation types among them: 68,281 Movie-Actor (MA), 148,502 Movie-User (MU) and 3,214 Movie-Director (MD). Movies (M) are categorized into four classes according to the genres: Comedy, Documentary, Drama, and Horror.
\item \textbf{MAG} is extracted from Microsoft Academic Graph, which contains 4,017 papers (P), 15,383 authors (A), 1,480 institutions (I) and 5,454 fields (F). All objects have attributes with 128-dimension features. It also contains four relation types: 3,880 Paper-Paper (PP), 40,378 Paper-Field (PF), 26,144 Paper-Author (PA) and 15,468 Author-Institution (AI). Papers (P) are divided into four classes based on the published venues: Astrophysics, IEEE Journal of Photovoltaics, Journal of Applied Meteorology and Climatology, and Low Temperature Physics.
\item \textbf{ACM} is a subgraph of ACM digital library, which contains 4,025 papers (P), 7,167 authors (A) and 60 subjects (S). All objects have 128-dimension features. There are two link types, i.e., 13,407 Paper-Author (PA) and 4,025 Paper-Subject (PS) between all kinds of objects. Papers (P), the target nodes are labeled as three classes: Computer Network, Data Mining and Database, according to their fields.
\end{itemize}

\section{Details of Baselines}
\label{sec:baseline}
We compare our HHGT model with nine baselines, including {\qy shallow model-based strategies and deep model-based methods.} The details of all baselines are shown as follows:
\begin{itemize}[leftmargin=*]
    \item \textbf{M2V}~\cite{dong2017metapath2vec}: employs meta-path based random walk and then utilizes skip-gram to embed an HG.
    \item \textbf{PTE}~\cite{tang2015pte}: first decomposes an HIN into a set of bipartite graphs where each describes only one edge type, and then learns the low-dimensional {\qy embeddings} for each bipartite network.
    \item \textbf{HIN2Vec}~\cite{fu2017hin2vec}: proposes to learn the latent embeddings of nodes and meta-paths in an HIN via undertaking multiple prediction training tasks jointly. 
    \item \textbf{ComplEx}~\cite{trouillon2016complex}: is a complex-valued embedding model in HINs, adept at capturing asymmetric relations and effectively modeling the interactions between {\qy nodes} and relations.
    \item \textbf{AspEm}~\cite{shi2018aspem}: first selects several aspects based on incompatibility measure and then learn embeddings for each  aspect. 
    % \item \textbf{AGAT}~\cite{liu2022aspect}: aims to adaptively learn the entity embeddings based on the prediction scenarios, achieved by enhancing GCNs through the integration of alternative learnable filters to incorporate both entity and relation information. 
    \item \textbf{HAN}~\cite{wang2019heterogeneous}: proposes an HGNN utilizing hierarchical attention, which includes both node-level and semantic-level attention. 
    % HAN leverages meta-paths to capture higher-order proximity instead of just considering direct neighbors.
    \item \textbf{R-GCN}~\cite{schlichtkrull2018modeling}: is the first GCN framework explicitly designed to solve the intricate multi-relational nature inherent in real-world HINs, i.e., utilizing multiple weight matrices to project the node embeddings into different relation spaces.
    \item \textbf{FastGTN}~\cite{yun2022graph}: captures task-specific multi-hop connections for node representations, avoiding the use of adjacency matrix multiplication in graph transformations.
    \item \textbf{SHGP}~\cite{yang2022self}: combines the structural clustering method with the attention-aggregation scheme so as to enhance the representation learning for HINs.
\end{itemize}

\section{Reproducibility} 
\label{sec:repro}
For all compared baselines, we employ their publicly released source code and adhere to the parameters recommended in their respective papers to ensure consistency. All the experiments are conducted on a  Linux (Ubuntu 18.04.6 LTS) server with one GPU (NVIDIA Tesla V100-SXM2) and two CPUs (Intel Xeon E5-2698 v4). Once our HHGT is trained, we can get all node {representations} via feed forward. Note that our \textit{Ring2Token} can be done offline, which offers the advantages of pre-computing and storing specific representations. Following previous studies~\cite{yang2022self,wang2019heterogeneous,zhao2020network} on HIN representation learning, we conduct two fundamental tasks for quantitative assessment: semi-supervised node classification and unsupervised node clustering.

\section{Additional Experimental Results}
\subsection{Embedding Visualization on ACM and IMDB Datasets} 
\label{sec:appendix_vis}

\begin{figure}[th]    
  \centering
  \subfloat[HHGT]{\label{fig:acm_HHGT}\parbox{0.12\textwidth}{\includegraphics[width=0.10\textwidth]{figure/acm_HHGT.png}}}
  \subfloat[SHGP]{\label{fig:acm_SHGP}\parbox{0.12\textwidth}{\includegraphics[width=0.10\textwidth]{figure/acm_SHGP.png}}}
  \subfloat[FastGTN]{\label{fig:acm_FAST}\parbox{0.12\textwidth}{\includegraphics[width=0.10\textwidth]{figure/acm_FAST.png}}}
  \subfloat[R-GCN]{\label{fig:acm_RGCN}\parbox{0.12\textwidth}{\includegraphics[width=0.10\textwidth]{figure/acm_RGCN.png}}}

  \subfloat[HAN]{\label{fig:acm_HAN}\parbox{0.12\textwidth}{\includegraphics[width=0.10\textwidth]{figure/acm_HAN.png}}}
  \subfloat[PTE]{\label{fig:acm_PTE}\parbox{0.12\textwidth}{\includegraphics[width=0.10\textwidth]{figure/acm_PTE.png}}}
  \subfloat[AspEm]{\label{fig:acm_AspEm}\parbox{0.12\textwidth}{\includegraphics[width=0.10\textwidth]{figure/acm_AspEm.png}}}
  \subfloat[HIN2Vec]{\label{fig:acm_HIN2Vec}\parbox{0.12\textwidth}{\includegraphics[width=0.10\textwidth]{figure/acm_HIN2Vec.png}}}

  \subfloat[M2V]{\label{fig:acm_M2V}\parbox{0.12\textwidth}{\includegraphics[width=0.10\textwidth]{figure/acm_M2V.png}}}
  \subfloat[ComplEx]{\label{fig:acm_ComplEx}\parbox{0.12\textwidth}{\includegraphics[width=0.10\textwidth]{figure/acm_ComplEx.png}}}

  % \captionsetup[subfloat]{captionskip=10pt}
  \caption{Embedding visualization on ACM dataset.}    
  \label{fig:vis_acm}  
\end{figure}

\begin{figure}[th]    
  \centering
  \subfloat[HHGT]{\label{fig:imdb_HHGT}\parbox{0.12\textwidth}{\includegraphics[width=0.10\textwidth]{figure/imdb_HHGT.png}}}
  \subfloat[SHGP]{\label{fig:imdb_SHGP}\parbox{0.12\textwidth}{\includegraphics[width=0.10\textwidth]{figure/imdb_SHGP.png}}}
  \subfloat[FastGTN]{\label{fig:imdb_FAST}\parbox{0.12\textwidth}{\includegraphics[width=0.10\textwidth]{figure/imdb_FAST.png}}}
  \subfloat[R-GCN]{\label{fig:imdb_RGCN}\parbox{0.12\textwidth}{\includegraphics[width=0.10\textwidth]{figure/imdb_RGCN.png}}}

  \subfloat[HAN]{\label{fig:imdb_HAN}\parbox{0.12\textwidth}{\includegraphics[width=0.10\textwidth]{figure/imdb_HAN.png}}}
  \subfloat[PTE]{\label{fig:imdb_PTE}\parbox{0.12\textwidth}{\includegraphics[width=0.10\textwidth]{figure/imdb_PTE.png}}}
  \subfloat[AspEm]{\label{fig:imdb_AspEm}\parbox{0.12\textwidth}{\includegraphics[width=0.10\textwidth]{figure/imdb_AspEm.png}}}
  \subfloat[HIN2Vec]{\label{fig:imdb_HIN2Vec}\parbox{0.12\textwidth}{\includegraphics[width=0.10\textwidth]{figure/imdb_HIN2Vec.png}}}

  \subfloat[M2V]{\label{fig:imdb_M2V}\parbox{0.12\textwidth}{\includegraphics[width=0.10\textwidth]{figure/imdb_M2V.png}}}
  \subfloat[ComplEx]{\label{fig:imdb_ComplEx}\parbox{0.12\textwidth}{\includegraphics[width=0.10\textwidth]{figure/imdb_ComplEx.png}}}
  
  \caption{Embedding visualization on IMDB dataset.}    
  \label{fig:vis_imdb}  
\end{figure}

We also visualize the learned {representations} on ACM and IMDB datasets. The findings presented in Figure~\ref{fig:vis_acm} and Figure~\ref{fig:vis_imdb} reveal {\qy two} noteworthy observations: (1) Deep model-based approaches demonstrate superior performance compared to most shallow model-based methods, as indicated by the highly dispersed and disordered pattern observed in the embedding visualization of the latter, suggesting an inferior overall visual quality. This discrepancy may be attributed to the fact that deep model-based strategies effectively {\qy model} complex HIN information through layer stacking, leading to improved performance.
% (1) The deep model-based models outperform most shallow mode-based ones, as evidenced by the highly scattered and disorganized pattern observed in the points of their embedding visualization, indicating a poor overall visual effect.  This discrepancy may be attributed to the fact that deep model-based models effectively capturing complex information within HINs through the stacking of multiple layers, resulting in improved performance.
(2) Our HHGT model stands out for its exceptional effectiveness, evident in its optimal within-class compactness and distinctly defined between-class boundaries.

\subsection{Parameter Study for Node Clustering Task}
\label{sec:para_clu}

\begin{figure}[h]    
  \centering          
  \subfloat[NMI]  {\label{fig:nclu_l_nmi}\includegraphics[width=0.23\textwidth]{figure/nclu_l_nmi.pdf}
  }
  \subfloat[ARI]{\label{fig:nclu_l_ari}\includegraphics[width=0.23\textwidth]{figure/nclu_l_ari.pdf}
  }
  \caption{Layer number study for node clustering.}    
  \label{fig:clu_L}  
\end{figure}

\noindent \textbf{Impact of Transformer Layer $L$.} We also assess the impact of layer number $L$ for node clustering task. We systematically vary $L$ within the set $\{1,2,3,4,5,6\}$ while keeping other parameters constant. As portrayed in Figure~\ref{fig:clu_L}, an initial elevation of the layer number $L$ contributes to enhanced performance, enabling the model to discern more intricate patterns. Remarkably, the model achieves its peak performance consistently at $L=2$ across all datasets. However, a subsequent growth in $L$ leads to a marginal downturn in performance, indicating a potential susceptibility to over-fitting and over-smoothing due to an excessively large model capacity.

\begin{figure}[h]    
  \centering          
  \subfloat[NMI]  {\label{fig:nclu_d_nmi}\includegraphics[width=0.23\textwidth]{figure/nclu_d_nmi.pdf}}
  \subfloat[ARI]{\label{fig:nclu_d_ari}\includegraphics[width=0.23\textwidth]{figure/nclu_d_ari.pdf}}
  \caption{Embedding size study for node clustering.}    
  \label{fig:clu_d}  
\end{figure}

\noindent \textbf{Impact of Embedding Size $d$.} 
To evaluate the effect of embedding dimension, we vary $d$ within the set $\{128, 256, 512, 1024, 2048\}$. Figure~\ref{fig:clu_d} presents the node clustering results across all datasets. As observed, in most cases, the model exhibits improved performance with larger embedding size. But we note that optimal results are not consistently achieved with higher-dimensional representations. For example, on the ACM dataset, the model attains the optimal NMI and ARI scores with $d=128$. This suggests that employing a higher-dimensional representation does not ensure the best performance across all scenarios.

\begin{figure}[h]    
  \centering          
  \subfloat[NMI]  {\label{fig:nclu_k_nmi}\includegraphics[width=0.23\textwidth]{figure/nclu_k_nmi.pdf}
  }
  \subfloat[ARI]{\label{fig:nclu_k_ari}\includegraphics[width=0.23\textwidth]{figure/nclu_k_ari.pdf}
  }
  \caption{Ring number study for node clustering.}    
  \label{fig:clu_K}  
\end{figure}

\noindent \textbf{Impact of Ring Number $K$.} 
We vary the {\zqy number of rings} $K$ from $1$ to $10$ to investigate its impact on node clustering task, and the results are depicted in Figure~\ref{fig:clu_K}. Notably, the model attains optimal performance with different values of $K$ on distinct datasets, specifically $K=6$ on MAG dataset and $K=7$ on both ACM and IMDB datasets. It indicates the adaptability of the model to diverse neighborhood configurations within different HINs. Furthermore, as $K$ increases, the performance gradually improves across all datasets, emphasizing the benefits of incorporating multiple $k$-ring information for node representation {\zqy learning} in HINs. However, after reaching a peak, further increments in $K$ result in a slight decline in performance. While a larger $K$ allows nodes to consider a broader neighborhood, excessively large values may encompass the entire network, introducing irrelevant information in the node's neighborhood and posing a potential risk of over-fitting.
